# Supplementary material for: Image-and-Spatial Transformer Networks for Structure-Guided Image Registration
Source: arXiv:1907.09200 source file (2019-07-22)
Supplement: Supplementary file 1 [file supplementary.tex]

% !TeX root=../paper.tex

\section{Supplementary Material}
\label{sec:supp}

\begin{figure}[t]
    \centering
    \includegraphics[width=\linewidth]{images/synthetic_seg.png}
    \caption{Figure for supplementary material.}
    \label{fig:synthetic-seg}
\end{figure}

\begin{figure}[t]
    \centering
    \includegraphics[width=\linewidth]{images/synthetic_pts.png}
    \caption{Figure for supplementary material.}
    \label{fig:synthetic-pts}
\end{figure}
